# Supplementary material for: Learning with Imperfect Models: When Multi-step Prediction Mitigates Compounding Error
Source: arXiv:2504.01766 source file (2025-04-02)
Supplement: Supplementary file 1 [file appendix.tex]

\onecolumn
%\tableofcontents
\begin{lemma}
    (Yassir's Lemma 2 but with inputs)
    Let $\{X_t\}_{t=1}^T$ evolve according to (1) with $C = I$ and $\Sigma_v = 0$.
Let $\Sigma_X = \mathbb{E}[\frac{1}{T} \sum_{t=1}^T X_tX_t^T]$ and choose arbitrary $\epsilon$ so that $0 < \epsilon < 1$. Then, for 
\[T \geq {\color{red} ??}\]
with probability at least $1-\delta$, 
    \[\lVert \Sigma_X^{-\frac{1}{2}}(\frac{1}{T}\sum_{t=1}^{T}X_tX_t^T)\Sigma_X^{-\frac{1}{2}} - I_{d_X}\rVert_{op}\leq \epsilon.\]
\end{lemma}
\begin{proof}
    
\end{proof}

\begin{lemma}
(from lemma a.8 of alcoi paper)
Let $\{\mathcal{F}_t\}_{t=0}^T$ be a filtration such that $\{Z_t\}_{t=1}^T$ is adapted to $\{\mathcal{F}_{t-1}\}_{t=0}^T$ with each $Z_t \in \mathbb{R}^{d_z}$ and $\{E_t\}_{t=1}^T$ is adapted to $\{\mathcal{F}_t\}_{t=0}^T$ where each $E_t \in \mathbb{R}$ is $\sigma_v^2$-conditionally sub-Gaussian. Let $\epsilon$ be a positive constant such that $\epsilon < 1$ and let $K\in \mathbb{R}$, $\Sigma \in \mathbb{R}^{d_z \times d_z}$ be such that 
\[\lVert \Sigma^{-\frac{1}{2}}\Bigl(\frac{1}{K}\sum_{t=1}^T Z_tZ_t^T\Bigl)\Sigma^{-\frac{1}{2}} - I_{d_z} \rVert_{op} \leq \epsilon. \]
Let $M \in \mathbb{R}^{d_z \times d_z}$. Then, for a fixed $\delta \in (0,1)$ with probability at least $1 - \delta$, 
\[\lVert M^T\Bigl(\frac{1}{K}\sum_{t=1}^T Z_tZ_t^T\Bigl)^{-1}\sum_{t=1}^TZ_tE_t \rVert^2 \leq \frac{2\sigma_v^2}{K(1-\epsilon)} \Bigl((1+\epsilon)\text{tr}( MM^T\Sigma^{-1})  + 2 \lVert MM^T\Sigma^{-1} \rVert\log(\frac{1}{\delta})\Bigl).\]
\end{lemma}
\begin{proof}

\begin{align*}
    &\lVert M^T(\sum_{t=1}^T Z_tZ_t^T\Bigl)^{-1}\sum_{t=1}^T Z_tE_t\Bigl\rVert_F^2 \\
    &= \lVert \Bigl(\sum_{t=1}^T M^{-1}Z_t(M^{-1}Z_t)^T\Bigl)^{-1}\sum_{t=1}^T M^{-1}Z_tE_t \rVert_F^2 \quad \text{{\color{red} Assuming M invertible (fix!)}}\\
    &= \lVert \Bigl((\sum_{t=1}^T M^{-1}Z_t(M^{-1}Z_t)^T)^2\Bigl)^{-\frac{1}{2}}\sum_{t=1}^T M^{-1}Z_tE_t  \rVert_F^2 \\
    &= 2\lVert \Bigl((\sum_{t=1}^T M^{-1}Z_t(M^{-1}Z_t)^T)^2 + (\sum_{t=1}^T M^{-1}Z_t(M^{-1}Z_t)^T)^2\Bigl)^{-\frac{1}{2}}\sum_{t=1}^T M^{-1}Z_tE_t  \rVert_F^2.
\end{align*}
By assumption, 
\[(1-\epsilon)\Sigma \preceq \frac{1}{K}\sum_{t=1}^TZ_tZ_t^T \preceq (1+\epsilon)\Sigma\]

which implies that 

\[(1-\epsilon)M^{-1}\Sigma (M^{-1})^T\preceq \frac{1}{K}M^{-1}\sum_{t=1}^TZ_tZ_t^T(M^{-1})^T \preceq (1+\epsilon)M^{-1}\Sigma(M^{-1})^T\]

and thus
\begin{align*}
    &(\sum_{t=1}^T M^{-1}Z_t(M^{-1}Z_t)^T)^2 + (\sum_{t=1}^T M^{-1}Z_t(M^{-1}Z_t)^T)^2 \\
    &\succeq ((1-\epsilon)M^{-1}K\Sigma (M^{-1})^T)^2 + \Bigl((1-\epsilon)M^{-1}K\Sigma (M^{-1})^T\Bigl)\Bigl(\sum_{t=1}^T M^{-1}Z_t(M^{-1}Z_t)^T\Bigl) \\
    &\succeq ((1-\epsilon)M^{-1}K\Sigma (M^{-1})^T)^2 + (1-\epsilon)\lambda_{min}\Bigl(M^{-1}K\Sigma (M^{-1})^T\Bigl)\Bigl(\sum_{t=1}^T M^{-1}Z_t(M^{-1}Z_t)^T\Bigl) \\
    &\succeq (1-\epsilon)^2\Bigl((M^{-1}K\Sigma (M^{-1})^T)^2 + \lambda_{min}\Bigl(M^{-1}K\Sigma (M^{-1})^T\Bigl)\Bigl(\sum_{t=1}^T M^{-1}Z_t(M^{-1}Z_t)^T\Bigl)\Bigl).
\end{align*}
Thus,
\begin{align*}
    &2\lVert  \Bigl((\sum_{t=1}^T M^{-1}Z_t(M^{-1}Z_t)^T)^2 + (\sum_{t=1}^T M^{-1}Z_t(M^{-1}Z_t)^T)^2\Bigl)^{-\frac{1}{2}} \sum_{t=1}^T M^{-1}Z_tE_t\rVert_{F}^2 \\
    &\leq \frac{2}{1-\epsilon}\lVert \Bigl((M^{-1}K\Sigma(M^{-1})^T)^2 + \lambda_{min}\Bigl(M^{-1}K\Sigma (M^{-1})^T\Bigl)\Bigl(\sum_{t=1}^T M^{-1}Z_t(M^{-1}Z_t)^T\Bigl)\Bigl)^{-\frac{1}{2}} \sum_{t=1}^T M^{-1}Z_tE_t\rVert_{F}^2 \\
    &= \frac{2}{1-\epsilon}\lambda_{min}\Bigl(M^{-1}K\Sigma (M^{-1})^T\Bigl)^{-1}\lVert  \Bigl(\frac{(M^{-1}K\Sigma (M^{-1})^T)^2}{\lambda_{min}\Bigl(M^{-1}K\Sigma(M^{-1})^T\Bigl)} + \Bigl(\sum_{t=1}^T M^{-1}Z_t(M^{-1}Z_t)^T\Bigl)\Bigl)^{-\frac{1}{2}} \sum_{t=1}^T M^{-1}Z_tE_t\rVert_{F}^2.
\end{align*}
Let $\hat{\Sigma} = \frac{(M^{-1}K\Sigma (M^{-1})^T)^2}{\lambda_{min}\Bigl(M^{-1}K\Sigma (M^{-1})^T\Bigl)}.$

Then by Theorem 4.1 of {\color{red} cite Ingvar's tutorial}, with probability $1-\delta$,
\begin{align*}
    &\frac{2}{1-\epsilon}\lambda_{min}\Bigl(M^{-1}K\Sigma (M^{-1})^T\Bigl)^{-1}\lVert \Bigl(\frac{(M^{-1}T\Sigma (M^{-1})^T)^2}{\lambda_{min}\Bigl(M^{-1}T\Sigma (M^{-1})^T\Bigl)} + \Bigl(\sum_{t=1}^T M^{-1}Z_t(M^{-1}Z_t)^T\Bigl)\Bigl)^{-\frac{1}{2}}\sum_{t=1}^T M^{-1}Z_tE_t \rVert_{F}^2 \\
    &\leq \frac{2}{1-\epsilon}\lambda_{min}\Bigl(M^{-1}K\Sigma (M^{-1})^T\Bigl)^{-1} \Bigl(\sigma_v^2 \log\det(I + M^{-1}\sum_{t=1}^T Z_tZ_t^T(M^{-1})^T\hat{\Sigma}^{-1})  + 2 \sigma_v^2\log(\frac{1}{\delta})\Bigl) \\
    &\leq \frac{2}{1-\epsilon}\lambda_{min}\Bigl(M^{-1}K\Sigma (M^{-1})^T\Bigl)^{-1} \Bigl(\sigma_v^2 \text{tr}( M^{-1}\sum_{t=1}^T Z_tZ_t^T(M^{-1})^T\hat{\Sigma}^{-1})  + 2 \sigma_v^2\log(\frac{1}{\delta})\Bigl) \\
    &\leq \frac{2}{1-\epsilon}\lambda_{min}\Bigl(M^{-1}K\Sigma (M^{-1})^T\Bigl)^{-1} \Bigl(\sigma_v^2 (1+\epsilon)\text{tr}( M^{-1}K \Sigma (M^{-1})^T\hat{\Sigma}^{-1})  + 2 \sigma_v^2\log(\frac{1}{\delta})\Bigl) \\
    &\leq \frac{2\sigma_v^2}{K(1-\epsilon)} \Bigl((1+\epsilon)\text{tr}( MM^T\Sigma^{-1})  + 2 \lVert MM^T\Sigma^{-1} \rVert\log(\frac{1}{\delta})\Bigl). \\
\end{align*}
\end{proof}

\begin{theorem}
(n step ahead error bound)

Let $\{Y_t\}_{t=1}^T$ evolve according to (1) with $C = I$ and $\Sigma_v = 0$. Let $\hat{G}$ be the multistep predictor (3) and let $\hat{Y}_{t+1:t+H}$ be the predicted trajectory
\[\hat{Y}_{t+1:t+H} = \hat{G}
\begin{bmatrix}
    X_t \\
    U_t \\
    \vdots \\
    U_{t+H-1}
\end{bmatrix}.\]
Let 
\[\Gamma = \begin{bmatrix}
    I \\
    A & I\\
    \vdots \\
    A^{H-1} & ... & A & I
\end{bmatrix}\]
Then, with probability at least $1 - \delta$ and for 
\[T \geq {\color{red} \text{burn in?}}\]
\begin{align*}
    &\Ex \Bigl[ \frac{1}{T-H} \sum_{t=1}^{T-H} \lVert Y_{t+1:t+H} - \hat{Y}_{t+1:t+H}\rVert^2\Bigl] \\
& \quad \leq \frac{2\sigma_v^2}{(T-H)(1-\epsilon)} \Bigl((1+\epsilon)(d_X + Hd_U) \tr (\Gamma^T\Gamma )  + 2 \lVert (I_{d_X + Hd_U} \otimes \Gamma^T\Gamma ) \rVert\log(\frac{1}{\delta})\Bigl)+\tr(\Gamma (I_H \otimes \Sigma_v)\Gamma^T).
\end{align*}

{\color{red} $\eps$ is arbitrary here, should we just set it to $\frac{1}{2}$? }
\end{theorem}

\begin{proof}

The rolled-out system dynamics are:
\[\begin{bmatrix}
    Y_{t+1} \\
    \vdots \\
    Y_{t+H}
\end{bmatrix} = 
\begin{bmatrix}
    A & B \\
    A^2  & AB & B \\
    A^H & A^{H-1}B & ... B
\end{bmatrix}
\begin{bmatrix}
    X_t \\
    U_t \\
    \vdots \\
    U_{t+H-1}
\end{bmatrix} + 
\begin{bmatrix}
    I \\
    A & I\\
    \vdots \\
    A^{H-1} & ... & A & I
\end{bmatrix}
\begin{bmatrix}
    W_t \\
    W_{t+1} \\
    \vdots \\
    W_{t+H-1}
\end{bmatrix}.\]
Let 
$G = \begin{bmatrix}
    A & B \\
    A^2  & AB & B \\
    A^H & A^{H-1}B & ...& B
\end{bmatrix}, 
Z_t = 
\begin{bmatrix}
    X_t \\
    U_t \\
    \vdots \\
    U_{t+H-1}
\end{bmatrix},
E_t = 
\begin{bmatrix}
    W_t \\
    W_{t+1} \\
    \vdots \\
    W_{t+H-1}
\end{bmatrix}.$

Then 
\begin{align*}
    &\Ex \Bigl[ \frac{1}{T-H} \sum_{t=1}^{T-H} \lVert Y_{t+1:t+H} - \hat{Y}_{t+1:t+H}\rVert^2\Bigl] \\
    &=\Ex \Bigl[ \frac{1}{T-H} \sum_{t=1}^{T-H} \lVert GZ_t + \Gamma E_t - \hat{G}Z_t\rVert^2\Bigl] \\
    &= \Ex \Bigl[ \frac{1}{T-H} \sum_{t=1}^{T-H} \lVert (G - \hat{G})Z_t\rVert^2 + \tr(\Gamma E_t E_t^T \Gamma^T)\Bigl] \\
    &= \Ex \Bigl[ \frac{1}{T-H} \sum_{t=1}^{T-H} \lVert (G - \hat{G})Z_t\rVert^2\Bigl]  + \tr(\Gamma (I_H \otimes \Sigma_w)\Gamma^T). 
\end{align*}
Let $\Sigma_Z = \Ex \Bigl[\frac{1}{T-H} \sum_{t=1}^{T-H} Z_tZ_t^T\Bigl]$. Then, 
\begin{align*}
    &\Ex \Bigl[ \frac{1}{T-H} \sum_{t=1}^{T-H} \lVert (G - \hat{G})Z_t \rVert^2\Bigl] \\
    &= \lVert (G - \hat{G})\Sigma_Z^{\frac{1}{2}}\rVert_F^2 \\
    &= \lVert \sum_{t=1}^{T-H}\Gamma E_tZ_t^T\Bigl(\sum_{t=1}^{T-H} Z_tZ_t^T\Bigl)^{-1}\Sigma_Z^{\frac{1}{2}}\rVert_F^2 \\
    &= \lVert \text{vec}\Bigl(\sum_{t=1}^{T-H}\Gamma E_tZ_t^T\Bigl(\sum_{t=1}^{T-H} Z_tZ_t^T\Bigl)^{-1}\Sigma_Z^{\frac{1}{2}}\Bigl)\rVert^2 \\
    &= \lVert (\Sigma_Z^{\frac{1}{2}} \otimes \Gamma )\text{vec}\Bigl(\sum_{t=1}^{T-H}E_tZ_t^T\Bigl(\sum_{t=1}^{T-H} Z_tZ_t^T\Bigl)^{-1}\Bigl)\rVert^2 \\
    &= \lVert (\Sigma_Z^{\frac{1}{2}} \otimes \Gamma )\Bigl(\sum_{t=1}^{T-H} (Z_t \otimes I_{Hd_X})(Z_t^T\otimes I_{Hd_X})\Bigl)^{-1}\sum_{t=1}^{T-H}(Z_t \otimes I_{Hd_X})E_t\rVert^2.
\end{align*}
Let $M = (\Sigma_Z^{\frac{1}{2}} \otimes \Gamma )^T$ and let $Z_t^i = Z_t \otimes e_i$ where $e_i$ is the $i$th column of $I_{Hd_X}$. Let $E_t^i$ be the $i$th coordinate of $E_t$. Then, 
\begin{align*}
    &\lVert (\Sigma_Z^{\frac{1}{2}} \otimes \Gamma )\Bigl(\sum_{t=1}^{T-H} (Z_t \otimes I_{Hd_X})(Z_t^T\otimes I_{Hd_X})\Bigl)^{-1}\sum_{t=1}^{T-H}(Z_t \otimes I_{Hd_X})E_t\rVert^2 \\
    &= \lVert M^T \Bigl(\sum_{t=1}^{T-H} \sum_i Z_t^i (Z_t^i)^T\Bigl)^{-1}\sum_{t=1}^{T-H} \sum_i Z_t^i E_t^i\rVert^2.
\end{align*}
Enumerate the $Z_t^i$ as $\{Z_t'\}_{t= 0}^{(T-H)Hd_X} = \{Z_1^1,...,Z_1^{Hd_X}, ..., Z_{T-H}^1,...,Z_{T-H}^{Hd_X}\}$. Similarly, let $\{E_t'\}_{t= 0}^{(T-H)Hd_X} = \{E_1^1,...,E_1^{Hd_X}, ..., E_{T-H}^1,...,E_{T-H}^{Hd_X}\}$. 
Then, 
\begin{align*}
    &\lVert M^T \Bigl(\sum_{t=1}^{T-H} \sum_i Z_t^i (Z_t^i)^T\Bigl)^{-1}\sum_{t=1}^{T-H} \sum_i Z_t^i E_t^i\rVert^2 \\
    &= \lVert M^T \Bigl(\sum_{t=1}^{(T-H)Hd_X}  Z_t' Z_t'^T\Bigl)^{-1}\sum_{t=1}^{(T-H)Hd_X} Z_t' E_t'\rVert^2.
\end{align*}

By Lemma 1  for $T \geq \text{\color{red} burn in (fix!)},$
\[\lVert \Sigma_Z^{-\frac{1}{2}}(\frac{1}{T-H}\sum_{t=1}^{T-H}Z_tZ_t^T)\Sigma_Z^{-\frac{1}{2}} - I_{d_X + Hd_U}\rVert_{op} \leq \epsilon\]
so using that 
\begin{align*}
    &\lVert (\Sigma_Z\otimes I_{Hd_X})^{-\frac{1}{2}}(\frac{1}{T-H}\sum_{t=1}^{(T-H)Hd_X}Z_t'Z_t'^T)(\Sigma_Z\otimes I_{Hd_X})^{-\frac{1}{2}} - I_{d_X + Hd_U}\otimes I_{Hd_X}\rVert_{op} \\
    &= \lVert (\Sigma_Z\otimes I_{Hd_X})^{-\frac{1}{2}}(\frac{1}{T-H}\sum_{t=1}^{T-H}(Z_{t}\otimes I_{Hd_X})(Z_{t}\otimes I_{Hd_X})^T)(\Sigma_Z\otimes I_{Hd_X})^{-\frac{1}{2}} - I_{d_X + Hd_U}\otimes I_{Hd_X}\rVert_{op} \\
    &= \lVert (\Sigma_Z^{-\frac{1}{2}}(\frac{1}{T-H}\sum_{t=1}^{T-H}Z_tZ_t^T)\Sigma_Z^{-\frac{1}{2}} - I_{d_X + Hd_U})\otimes I_{Hd_X}\rVert_{op} \\
    &\leq \lVert (\Sigma_Z^{-\frac{1}{2}}(\frac{1}{T-H}\sum_{t=1}^{T-H}Z_tZ_t^T)\Sigma_Z^{-\frac{1}{2}} - I_{d_X + Hd_U})\rVert_{op}\lVert I_{Hd_X}\rVert_{op} \\
    &\leq \epsilon. 
\end{align*}
Thus, we can conclude by Lemma 2 that 
\begin{align*}
    &\lVert M^T \Bigl(\sum_{t=1}^{(T-H)Hd_X}  Z_t' Z_t'^T\Bigl)^{-1}\sum_{t=1}^{(T-H)Hd_X} Z_t' E_t'\rVert^2 \\
    &\leq \frac{2\sigma_v^2}{(T-H)(1-\epsilon)} \Bigl((1+\epsilon)\text{tr}( MM^T(\Sigma_Z\otimes I_{Hd_X})^{-1})  + 2 \lVert MM^T(\Sigma_Z\otimes I_{Hd_X})^{-1} \rVert\log(\frac{1}{\delta})\Bigl) \\
    &= \frac{2\sigma_v^2}{(T-H)(1-\epsilon)} \Bigl((1+\epsilon)\text{tr}( (\Sigma_Z^{\frac{1}{2}} \otimes \Gamma )^T(\Sigma_Z^{\frac{1}{2}} \otimes \Gamma )(\Sigma_Z\otimes I_{Hd_X})^{-1})  + 2 \lVert (\Sigma_Z^{\frac{1}{2}} \otimes \Gamma )^T(\Sigma_Z^{\frac{1}{2}} \otimes \Gamma )(\Sigma_Z\otimes I_{Hd_X})^{-1} \rVert\log(\frac{1}{\delta})\Bigl) \\
    &= \frac{2\sigma_v^2}{(T-H)(1-\epsilon)} \Bigl((1+\epsilon)\text{tr}( (\Sigma_Z \otimes \Gamma^T\Gamma )(\Sigma_Z\otimes I_{Hd_X})^{-1})  + 2 \lVert (\Sigma_Z \otimes \Gamma^T\Gamma )(\Sigma_Z\otimes I_{Hd_X})^{-1} \rVert\log(\frac{1}{\delta})\Bigl) \\
    &= \frac{2\sigma_v^2}{(T-H)(1-\epsilon)} \Bigl((1+\epsilon)\text{tr} (I_{d_X + Hd_U} \otimes \Gamma^T\Gamma )  + 2 \lVert (I_{d_X + Hd_U} \otimes \Gamma^T\Gamma ) \rVert\log(\frac{1}{\delta})\Bigl) \\
    &= \frac{2\sigma_v^2}{(T-H)(1-\epsilon)} \Bigl((1+\epsilon)(d_X + Hd_U)\text{tr} (\Gamma^T\Gamma )  + 2 \lVert (I_{d_X + Hd_U} \otimes \Gamma^T\Gamma ) \rVert\log(\frac{1}{\delta})\Bigl).
\end{align*}
\end{proof}

\begin{theorem}
    (one step rollout)
    Let $\{Y_t\}_{t=1}^T$ evolve according to system dynamics \ref{eq: dynamics} with $C = I$ and $\Sigma_v = 0$. Let $\bmat{\hat G_y & \hat G_u}$ be the one step predictor \ref{eq: single step LS} and let $\hat{X}_{t+1:t+H}$ be the predicted trajectory according to the one step rollout as described in \ref{eq: single step rollout}.

Let 
\[\Gamma = \begin{bmatrix}
    I \\
    A & I\\
    \vdots \\
    A^{H-1} & ... & A & I
\end{bmatrix}, \Lambda = \begin{bmatrix}
    I \\
     & B\\
    & &\ddots\\
     &  & & B
\end{bmatrix}\] and let 
\[K_1 = I_H \otimes \bmat{I_{d_x} \\ 0_{d_u \times d_x}}, K_2 = \bmat{ I_{d_x +(H-1)d_u} & 0_{d_x +(H-1)d_u \times d_u}}, K_3 = (I_H \otimes \bmat{0_{d_x \times  d_u} \\ I_{d_u}})\bmat{0_{Hd_u \times d_x} & I_{Hd_u}}.\]

Then, with probability at least $1 - \delta$ and for 
\[T \geq {\color{red} \text{burn in?}}\]
\begin{align*}
    &\Ex \Bigl[ \frac{1}{T-H} \sum_{t=1}^{T-H} \lVert Y_{t+1:t+H} - \hat{Y}_{t+1:t+H}\rVert^2\Bigl] \\
    &\quad \leq \frac{2\sigma_v^2}{T(1-\epsilon)} \Bigl((1+\epsilon)\text{tr}((K_1 \Gamma \Lambda K_2 + K_3)\Sigma_Z(K_1 \Gamma \Lambda K_2 + K_3)^T(I_H \otimes \Sigma)^{-1}) \text{tr}(\Gamma^T\Gamma) \\
    &\quad \quad \quad + 2 \lVert (K_1 \Gamma \Lambda K_2 + K_3)\Sigma_Z(K_1 \Gamma \Lambda K_2 + K_3)^T(I_H \otimes \Sigma)^{-1} \otimes \Gamma^T\Gamma \rVert\log(\frac{1}{\delta})\Bigl) +\tr(\Gamma (I_H \otimes \Sigma_v)\Gamma^T)
\end{align*}

where $\Sigma_Z = \Ex \Bigl[ \frac{1}{T-H} \sum_{t=1}^{T-H} \begin{bmatrix}
    Y_t \\
    U_t \\
    \vdots \\
    U_{t+H-1}
\end{bmatrix}\begin{bmatrix}
    Y_t \\
    U_t \\
    \vdots \\
    U_{t+H-1}
\end{bmatrix}^T\Bigl]$ and $\Sigma = \Ex \Bigl[ \frac{1}{T} \sum_{t=1}^{T} \bmat{X_t \\ U_t}\bmat{X_t \\ U_t}^T\Bigl]$.

\end{theorem}
\begin{proof}
The rolled-out system dynamics are:
\[\begin{bmatrix}
    Y_{t+1} \\
    \vdots \\
    Y_{t+H}
\end{bmatrix} = 
\begin{bmatrix}
    A & B \\
    A^2  & AB & B \\
    A^H & A^{H-1}B & ... B
\end{bmatrix}
\begin{bmatrix}
    Y_t \\
    U_t \\
    \vdots \\
    U_{t+H-1}
\end{bmatrix} + 
\begin{bmatrix}
    I \\
    A & I\\
    \vdots \\
    A^{H-1} & ... & A & I
\end{bmatrix}
\begin{bmatrix}
    W_t \\
    W_{t+1} \\
    \vdots \\
    W_{t+H-1}
\end{bmatrix}.\]
The predicted trajectory is given by 
\[\begin{bmatrix}
    \hat Y_{t+1} \\
    \vdots \\
   \hat Y_{t+H}
\end{bmatrix} = 
\bmat{\hat G_y & \hat G_u & 0 & \dots & 0 \\
                   \hat G_y^2 & \hat G_y \hat G_u & \hat G_u   &\dots & 0 \\
                   \vdots  &&& \ddots \\
                   \hat G_y^{H} &   \hat G_y^{H-1}\hat G_u &  \hat G_y^{H-2}\hat G_u &\dots & \hat G_u \\}
\begin{bmatrix}
    Y_t \\
    U_t \\
    \vdots \\
    U_{t+H-1}
\end{bmatrix} .\]
Let $Z_t = 
\begin{bmatrix}
    Y_t \\
    U_t \\
    \vdots \\
    U_{t+H-1}
\end{bmatrix}$ and
$E_t = 
\begin{bmatrix}
    W_t \\
    W_{t+1} \\
    \vdots \\
    W_{t+H-1}
\end{bmatrix}$. Then, 
\begin{align*}
    &\Ex \Bigl[ \frac{1}{T-H} \sum_{t=1}^{T-H} \lVert Y_{t+1:t+H} - \hat{Y}_{t+1:t+H}\rVert^2\Bigl] \\
    &= \Ex \Bigl[ \frac{1}{T-H} \sum_{t=1}^{T-H} \lVert 
    \bmat{ A - \hat G_y & B - \hat G_u & 0 & \dots & 0 \\
                  A^2 - \hat G_y^2 & AB - \hat G_y \hat G_u & B - \hat G_u   &\dots & 0 \\
                   \vdots  &&& \ddots \\
                  A^{H} - \hat G_y^{H} &  A^{H-1} B -  \hat G_y^{H-1}\hat G_u &  A^{H-2} B - \hat G_y^{H-2}\hat G_u &\dots & B -\hat G_u \\} Z_t + \Gamma
E_t\rVert^2\Bigl] \\
&= \Ex \Bigl[ \frac{1}{T-H} \sum_{t=1}^{T-H} \lVert \bmat{ A - \hat G_y & B - \hat G_u & 0 & \dots & 0 \\
                  A^2 - \hat G_y^2 & AB - \hat G_y \hat G_u & B - \hat G_u   &\dots & 0 \\
                   \vdots  &&& \ddots \\
                  A^{H} - \hat G_y^{H} &  A^{H-1} B -  \hat G_y^{H-1}\hat G_u &  A^{H-2} B - \hat G_y^{H-2}\hat G_u &\dots & B -\hat G_u \\}Z_t\rVert^2 + \tr(\Gamma E_t E_t^T \Gamma^T)\Bigl] \\
&= \Ex \Bigl[ \frac{1}{T-H} \sum_{t=1}^{T-H} \lVert \bmat{ A - \hat G_y & B - \hat G_u & 0 & \dots & 0 \\
                  A^2 - \hat G_y^2 & AB - \hat G_y \hat G_u & B - \hat G_u   &\dots & 0 \\
                   \vdots  &&& \ddots \\
                  A^{H} - \hat G_y^{H} &  A^{H-1} B -  \hat G_y^{H-1}\hat G_u &  A^{H-2} B - \hat G_y^{H-2}\hat G_u &\dots & B -\hat G_u \\}Z_t\rVert^2\Bigl]  + \tr(\Gamma (I_H \otimes \Sigma_w)\Gamma^T).
\end{align*}

Let $\Sigma_Z = \Ex \Bigl[\frac{1}{T-H} \sum_{t=1}^{T-H} Z_tZ_t^T\Bigl]$. Then, 
\begin{align*}
    &\Ex \Bigl[ \frac{1}{T-H} \sum_{t=1}^{T-H} \lVert \bmat{ A - \hat G_y & B - \hat G_u & 0 & \dots & 0 \\
                  A^2 - \hat G_y^2 & AB - \hat G_y \hat G_u & B - \hat G_u   &\dots & 0 \\
                   \vdots  &&& \ddots \\
                  A^{H} - \hat G_y^{H} &  A^{H-1} B -  \hat G_y^{H-1}\hat G_u &  A^{H-2} B - \hat G_y^{H-2}\hat G_u &\dots & B -\hat G_u \\}Z_t\rVert^2\Bigl] \\
    &=  \lVert \bmat{ A - \hat G_y & B - \hat G_u & 0 & \dots & 0 \\
                  A^2 - \hat G_y^2 & AB - \hat G_y \hat G_u & B - \hat G_u   &\dots & 0 \\
                   \vdots  &&& \ddots \\
                  A^{H} - \hat G_y^{H} &  A^{H-1} B -  \hat G_y^{H-1}\hat G_u &  A^{H-2} B - \hat G_y^{H-2}\hat G_u &\dots & B -\hat G_u \\}\Sigma_Z^{\frac{1}{2}}\rVert_F^2.
\end{align*}

Note that \[A^k B - \hat G_y^k \hat G_u = (A^k - \hat G_y^k)B - (A^k - \hat G_y^k)(B - \hat G_u) + A^k(B - \hat G_u)\] and that for $k>1$,
\[A^k - \hat G_y^k = \sum_{i=0}^{k-1} A^{k-i-1}(A - \hat G_y)A^i - \hat G_y^{k-2}(A - \hat G_y)^2\]
so that 
\[A^k B - \hat G_y^k\hat G_u = \sum_{i=0}^{k-1} A^{k-i-1}(A - \hat G_y)A^iB + A^k(B - \hat G_u) + \hat G_y^{k-2}(A - \hat G_y)^2 \hat G_u - (\sum_{i=0}^{k-1} A^{k-i-1}(A - \hat G_y)A^i )(B-\hat G_u).\]

These identities give that 
\[\bmat{ A - \hat G_y & B - \hat G_u & 0 & \dots & 0 \\
                  A^2 - \hat G_y^2 & AB - \hat G_y \hat G_u & B - \hat G_u   &\dots & 0 \\
                   \vdots  &&& \ddots \\
                  A^{H} - \hat G_y^{H} &  A^{H-1} B -  \hat G_y^{H-1}\hat G_u &  A^{H-2} B - \hat G_y^{H-2}\hat G_u &\dots & B -\hat G_u \\} = F_1 +F_2\]

where 
\[F_1 = \bmat{ A - \hat G_y & B - \hat G_u & 0 & \dots & 0 \\
                  A(A - \hat G_y) + (A - \hat G_y)A & (A - \hat G_y)B + A(B - \hat G_u) & B - \hat G_u   &\dots & 0 \\
                   \vdots  &&& \ddots \\
                  \sum_{i=0}^{H-1} A^{k-i-1}(A - \hat G_y)A^i &  \sum_{i=0}^{H-2} A^{k-i-1}(A - \hat G_y)A^i B + A^{H-1}(B - \hat G_u) &   &\dots & B -\hat G_u \\}\]
consists of low order terms and 
\[F_2 = \bmat{ 0 & 0 & 0 & \dots & 0 \\
                  (A - \hat G_y)^2 & -(A - \hat G_y)(B - \hat G_u) & 0   &\dots & 0 \\
                   \vdots  &&& \ddots \\
                  \hat G_y^{H-2}(A - \hat G_y)^2 & \hat G_y^{H-3}(A - \hat G_y)^2\hat G_u -  \sum_{i=0}^{H-2} A^{H+i-2}(A - \hat G_y)A^i(B - \hat G_u)  & & \dots & 0 \\}\]
consists of higher powers of $(A-\hat G_y)$ and cross terms $(A - \hat G_y)(B - \hat G_u)$. Then,
\begin{align*}
    & \lVert \bmat{ A - \hat G_y & B - \hat G_u & 0 & \dots & 0 \\
                  A^2 - \hat G_y^2 & AB - \hat G_y \hat G_u & B - \hat G_u   &\dots & 0 \\
                   \vdots  &&& \ddots \\
                  A^{H} - \hat G_y^{H} &  A^{H-1} B -  \hat G_y^{H-1}\hat G_u &  A^{H-2} B - \hat G_y^{H-2}\hat G_u &\dots & B -\hat G_u \\}\Sigma_Z^{\frac{1}{2}}\rVert_F^2 \\
    &= \lVert (F_1 + F_2)\Sigma_Z^{\frac{1}{2}}\rVert_F^2 \\
    &\leq \Bigl( \lVert (F_1)\Sigma_Z^{\frac{1}{2}}\rVert_F + \lVert (F_2)\Sigma_Z^{\frac{1}{2}}\rVert_F \Bigl)^2
\end{align*}
{\color{red} Disregarding $F_2$ here but need to find a burn-in to justify doing this}

Note that 
\begin{align*}
    F_1 &= \Gamma \Bigl((I_H \otimes (A - \hat G_y)) \Gamma \Lambda \bmat{ I_{d_x +(H-1)d_u} & 0_{d_x +(H-1) d_u\times d_u}} + (I_H \otimes (B - \hat G_u)) \bmat{0_{H d_u \times d_x} & I_{Hd_u}} \Bigl) \\
    &= \Gamma \Bigl(I_H \otimes \bmat{A - \hat G_y & B - \hat G_u}\Bigl)\Bigl((I_H \otimes \bmat{I_{d_x} \\ 0_{d_u \times d_x}}) \Gamma \Lambda \bmat{ I_{d_x +(H-1)d_u} & 0_{d_x +(H-1) d_u\times d_u}} + (I_H \otimes \bmat{0_{d_x \times d_u} \\ I_{d_u}})\bmat{0_{H d_u \times d_x} & I_{Hd_u}}\Bigl)
\end{align*}

Thus, 
\begin{align*}
    &\lVert F_1\Sigma_Z^{\frac{1}{2}}\rVert_F^2 \\
    &= \norm{\Gamma \Bigl(I_H \otimes \bmat{A - \hat G_y & B - \hat G_u}\Bigl)\Bigl((I_H \otimes \bmat{I_{d_x} \\ 0_{d_u \times d_x}}) \Gamma \Lambda \bmat{ I_{d_x +(H-1)d_u} & 0_{d_x +(H-1) d_u\times d_u}} + (I_H \otimes \bmat{0_{d_x \times d_u} \\ I_{d_u}})\bmat{0_{H d_u \times d_x} & I_{Hd_u}}\Bigl)\Sigma_Z^{\frac{1}{2}}}_F^2 \\
    &= \norm{\Bigl(\Sigma_Z^{\frac{1}{2}}\Bigl((I_H \otimes \bmat{I_{d_x} \\ 0_{d_u \times d_x}}) \Gamma \Lambda \bmat{ I_{d_x +(H-1)d_u} & 0_{d_x +(H-1) d_u\times d_u}} + (I_H \otimes \bmat{0_{d_x \times d_u} \\ I_{d_u}})\bmat{0_{H d_u \times d_x} & I_{Hd_u}}\Bigl)^T \otimes \Gamma \Bigl) \VEC{ \Bigl(I_H \otimes \bmat{A - \hat G_y & B - \hat G_u}\Bigl)}}^2 \\
    &= \norm{M^T\VEC{ \Bigl(I_H \otimes \bmat{A - \hat G_y & B - \hat G_u}\Bigl)}}^2
\end{align*}
where we set $M = \Bigl(\Sigma_Z^{\frac{1}{2}}\Bigl((I_H \otimes \bmat{I_{d_x} \\ 0_{d_u \times d_x}}) \Gamma \Lambda \bmat{ I_{d_x +(H-1)d_u} & 0_{d_x +(H-1) d_u\times d_u}} + (I_H \otimes \bmat{0_{d_x \times d_u} \\ I_{d_u}})\bmat{0_{H d_u \times d_x} & I_{Hd_u}}\Bigl)^T \otimes \Gamma \Bigl)^T$.

Note that 
\[\bmat{A - \hat G_y & B - \hat G_u} = \sum_{t=1}^T W_t \bmat{X_t \\ U_t}^T \Bigl(\sum_{t=1}^T\bmat{X_t \\ U_t}\bmat{X_t \\ U_t}^T\Bigl)^{-1}\]
so that 
\begin{align*}
    &\VEC{ \Bigl(I_H \otimes \bmat{A - \hat G_y & B - \hat G_u}\Bigl)} \\
    &= \VEC{ \Bigl(I_H \otimes \sum_{t=1}^T W_t \bmat{X_t \\ U_t}^T \Bigl(\sum_{t=1}^T\bmat{X_t \\ U_t}\bmat{X_t \\ U_t}^T\Bigl)^{-1}\Bigl)} \\
    &= \VEC{ \Bigl( \sum_{t=1}^T (I_H \otimes W_t) (I_H \otimes \bmat{X_t \\ U_t})^T \Bigl(\sum_{t=1}^T (I_H \otimes \bmat{X_t \\ U_t})(I_H \otimes \bmat{X_t \\ U_t})^T\Bigl)^{-1}\Bigl)} \\
    &=   \Bigl(\sum_{t=1}^T (I_H \otimes \bmat{X_t \\ U_t} \otimes I_{Hd_X})(I_H \otimes \bmat{X_t \\ U_t})^T \otimes I_{Hd_X}\Bigl)^{-1}\sum_{t=1}^T (I_H \otimes \bmat{X_t \\ U_t} \otimes I_{Hd_X}) \VEC{(I_H \otimes W_t)}.
\end{align*}
Let $Z_t^{ij} = \bmat{X_t \\ U_t} \otimes e_i \otimes e_j$ where $e_i$ is the $i$th column of $I_{H}$ and $e_j$ is the $j$th column of $I_{Hd_X}$. Let $W_t^{ij}$ enumerate the elements of  $\VEC{(I_H \otimes W_t)}$. Then, 
\begin{align*}
    &\Bigl(\sum_{t=1}^T (I_H \otimes \bmat{X_t \\ U_t} \otimes I_{Hd_X})(I_H \otimes \bmat{X_t \\ U_t})^T \otimes I_{Hd_X}\Bigl)^{-1}\sum_{t=1}^T (I_H \otimes \bmat{X_t \\ U_t} \otimes I_{Hd_X}) \VEC{(I_H \otimes W_t)} \\
    &= \Bigl(\sum_{t=1}^T \sum_{i=1}^H \sum_{j=1}^{Hd_X} Z_t^{ij}(Z_t^{ij})^T \Bigl)^{-1} \sum_{t=1}^T \sum_{i=1}^H \sum_{j=1}^{Hd_X} Z_t^{ij}W_t^{ij}.
\end{align*}
Enumerate the $Z_t^{ij}$ as $\{Z_t'\}_{t= 0}^{TH^2d_X} = \{Z_1^{1,1},...,Z_1^{H,1}, ..., Z_{T}^{1,1},...,Z_{T}^{H,1},...,Z_1^{1,Hd_X},...,Z_1^{H,Hd_X}, ..., Z_{T}^{1,d_X},...,Z_{T}^{H,Hd_X}\}$. Similarly, let $\{W_t'\}_{t= 0}^{TH^2d_X} = \{W_1^{1,1},...,W_1^{H,1}, ..., W_{T}^{1,1},...,W_{T}^{H,1}, ...,W_1^{1,Hd_X},...,W_1^{H,Hd_X}, ..., W_{T}^{1,Hd_X},...,W_{T}^{H,Hd_X}\}$.

Then, 
\begin{align*}
    &\lVert M^T \Bigl(\sum_{t=1}^T \sum_{i=1}^H \sum_{j=1}^{Hd_X} Z_t^{ij}(Z_t^{ij})^T \Bigl)^{-1} \sum_{t=1}^T \sum_{i=1}^H \sum_{j=1}^{Hd_X} Z_t^{ij}W_t^{ij}\rVert^2 \\
    &= \lVert M^T \Bigl(\sum_{t=1}^{TH^2d_X}  Z_t' Z_t'^T\Bigl)^{-1}\sum_{t=1}^{TH^2d_X} Z_t' W_t'\rVert^2.
\end{align*}

By Lemma 1  for $T \geq \text{\color{red} burn in (fix!)},$
\[\lVert \Sigma^{-\frac{1}{2}}(\frac{1}{T}\sum_{t=1}^{T}\bmat{X_t \\ U_t}\bmat{X_t \\ U_t}^T)\Sigma^{-\frac{1}{2}} - I_{d_X + d_U}\rVert_{op} \leq \epsilon\]
so using that 
\begin{align*}
    &\lVert (I_H \otimes\Sigma \otimes I_{Hd_X})^{-\frac{1}{2}}(\frac{1}{T}\sum_{t=1}^{TH^2d_X}Z_t'Z_t'^T)(I_H \otimes \Sigma \otimes I_{Hd_X})^{-\frac{1}{2}} - I_H \otimes I_{d_X + d_U}\otimes I_{Hd_X}\rVert_{op} \\
    &= \lVert (I_H \otimes \Sigma \otimes I_{Hd_X})^{-\frac{1}{2}}(\frac{1}{T}\sum_{t=1}^{T}(I_H \otimes \bmat{X_t \\ U_t} \otimes I_{Hd_X})(I_H \otimes \bmat{X_t \\ U_t} \otimes I_{Hd_X})^T)(\Sigma \otimes I_{Hd_X})^{-\frac{1}{2}} - I_H \otimes I_{d_X + d_U}\otimes I_{Hd_X}\rVert_{op} \\
    &= \lVert I_H \otimes (\Sigma^{-\frac{1}{2}}(\frac{1}{T}\sum_{t=1}^{T}\bmat{X_t \\ U_t}\bmat{X_t \\ U_t}^T)\Sigma^{-\frac{1}{2}} - I_{d_X + d_U})\otimes I_{Hd_X}\rVert_{op} \\
    &\leq \lVert I_{H}\rVert_{op}\lVert (\Sigma^{-\frac{1}{2}}(\frac{1}{T-H}\sum_{t=1}^{T}\bmat{X_t \\ U_t}\bmat{X_t \\ U_t}^T)\Sigma^{-\frac{1}{2}} - I_{d_X + d_U})\rVert_{op}\lVert I_{Hd_X}\rVert_{op} \\
    &\leq \epsilon. 
\end{align*}
Thus, we can conclude by Lemma 2 that 
\begin{align*}
    \lVert M^T \Bigl(\sum_{t=1}^{TH^2d_X}  Z_t' Z_t'^T\Bigl)^{-1}\sum_{t=1}^{TH^2d_X} Z_t' W_t'\rVert^2 \leq \frac{2\sigma_v^2}{T(1-\epsilon)} \Bigl((1+\epsilon)\text{tr}( MM^T(I_H \otimes\Sigma \otimes I_{Hd_X})^{-1})  + 2 \lVert MM^T(I_H \otimes\Sigma \otimes I_{Hd_X})^{-1} \rVert\log(\frac{1}{\delta})\Bigl).
\end{align*}
\end{proof}
